# Supplementary material for: SR-LLM: Rethinking the Structured Representation in Large Language Model
Source: arXiv:2502.14352 source file (2025-02-20)
Supplement: Supplementary file 1 [file appendix_old.tex]

\appendix
\section{Appendix}
You may include other additional sections here.

\subsection{PST-to-NLD}
\paragraph{Definition of PST.}
% \begin{enumerate}
    % \item \textbf{Definition of PST} \\
    PST is represented as a tree structure \( T = (N, E) \). Here \( N \) denotes the set of nodes, representing the syntactic components of a sentence (e.g., part-of-speech tags and phrase labels). Node types include \( S \) (sentence), \( NP \) (noun phrase), \( VP \) (verb phrase), etc.  \( E \) denotes the set of edges, representing dependencies between components.
    An example of the original PST structure is shown in the Figure~\ref{fig:sr2nld}.

\paragraph{Conversion of PST to a Linear Structure Using Depth-First Search (DFS).}
    % \item \textbf{Conversion of PST to a Linear Structure Using Depth-First Search (DFS)} \\
    Starting from the root node (typically \( n_0 \), representing the sentence's syntactic structure, such as \( S \)), we traverse the tree in a depth-first search (DFS) manner, converting it into a linear sequence of symbols \( P \).
    
    % \begin{equation}
    %     P = (S, (NP, (NNP, John)), (VP, (VBD, saw), (NP, (DT, a), (NN, dog))))
    % \end{equation}

\paragraph{Mapping PST Identifiers to Natural Language Descriptions.}
    % \item \textbf{Mapping PST Identifiers to Natural Language Descriptions} \\
    We define a mapping function \( M \) to translate each identifier (e.g., \( S \), \( NP \), \( VBD \)) and its child nodes into natural language descriptions. The dictionary \( D \), which specifies the natural language interpretation of each identifier, is detailed in the appendix. For each triplet \( (n, c_1, c_2) \), where \( n \) is a node and \( c_1 \), \( c_2 \) are its children, we apply the mapping function \( M(n) = \text{description}(n) \). The resulting natural language description \( S \) is as follows:
    
    % \begin{equation}
    %     S = (Sentence (Noun Phrase (Proper noun, singular John)) (Verb Phrase (Verb, past tense saw) (Noun Phrase (Determiner a) (Noun, singular or mass dog))))
    % \end{equation}
    
\paragraph{Refinement of Natural Language Descriptions Using a Language Model.}
    % \item \textbf{Refinement of Natural Language Descriptions Using a Language Model} \\
    To make the descriptions more natural and coherent, the generated descriptions \( S \) are refined using the language model \( F_{\text{LM}}: S \rightarrow S_{\text{refined}} \). The specific prompts and the refined results are detailed in the appendix. 
    % For example:
    % \begin{itemize}
    %   \item \textbf{Original sentence}: John saw a dog.
    %   \item \textbf{Grammatical structure}:
    %   \begin{itemize}
    %       \item \textbf{John}: Noun phrase, the subject of the sentence, referring to the person "John."
    %       \item \textbf{saw}: Verb phrase, indicating the past action performed by the subject, which is the act of seeing.
    %       \item \textbf{a dog}: Noun phrase, the direct object of the sentence, specifying what was seen, which is "a dog."
    %   \end{itemize}
    % \end{itemize}
% \end{enumerate}

\begin{figure}
\centering
\vspace{0.1in}
\includegraphics[width=0.7\linewidth]{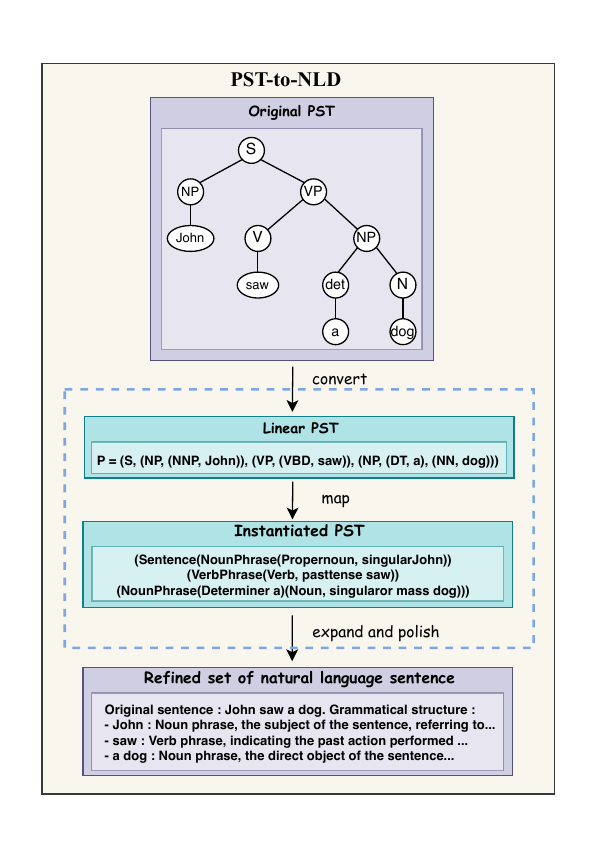}
\vspace{0.1in}
\caption{ PST-to-NLD.}
\label{fig:pst2nld}
\vspace{0.1in}
\end{figure}

\begin{figure}
\centering
\vspace{0.1in}
\includegraphics[width=0.7\linewidth]{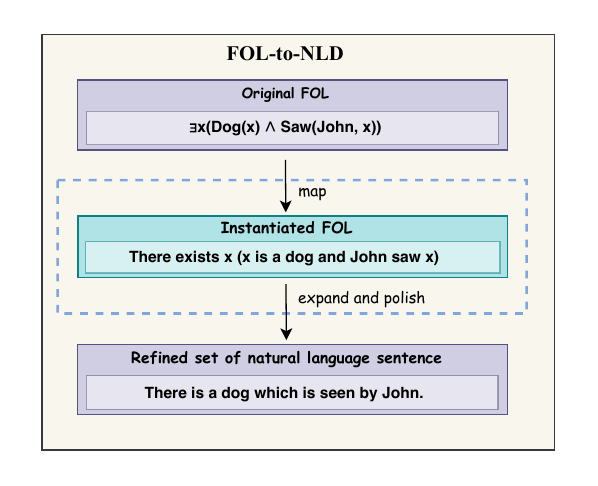}
\vspace{0.1in}
\caption{ FOL-to-NLD.}
\label{fig:fol2nld}
\vspace{0.1in}
\end{figure}

\subsection{FOL-to-NLD}
\paragraph{Definition of FOL.}
% \begin{enumerate}
    % \item \textbf{Definition of FOL} \\
    FOL is represented as \( F = (Q, V, P, C) \), where 
    % \begin{itemize}
         \( Q \) denotes the set of quantifiers, used to express the existence of variables, such as \( \exists \) (exists) and \( \forall \) (for all).
         \( V \) represents the set of variables, representing objects in FOL, typically denoted as \( x, y, z \).
         \( P \) represents the set of predicates, used to express properties of objects or relationships between multiple objects.
         \( C \) represents the set of logical connectives, used to connect multiple propositions, including conjunction (\( \land \)), disjunction (\( \lor \)), and negation (\( \neg \)).
    % \end{itemize}
    An example of the original FOL structure is shown in the Figure~\ref{fig:sr2nld}.

\paragraph{Mapping FOL to Natural Language Descriptions.}
    % \item \textbf{Mapping FOL to Natural Language Descriptions} \\
    We define a mapping function \( M = (D, L) \), where
    % \begin{itemize}
         \( D \) is a set of symbol mappings that translates variables, predicates, and logical operators in FOL into natural language descriptions.
         \( L \) is a set of logical mapping rules that transforms the logical structure of FOL into natural language syntax.
    % \end{itemize}\
    By applying these mapping rules to the initial FOL expressions, we can convert logical symbols into natural language descriptions.
    
\paragraph{Refinement of Natural Language Descriptions Using a Language Model.}
    % \item \textbf{Refinement of Natural Language Descriptions Using a Language Model} \\
    To ensure that the descriptions are coherent and fluent, we refine the generated descriptions \( S \) using the language model \( F_{\text{LM}}: S \rightarrow S_{\text{refined}} \). The specific prompts and refined descriptions are detailed in the appendix. 
    % For example:
    % \begin{itemize}
    %    \item \textbf{Original logic expression}:
    %   \exists x(Dog(x) \land Saw(John, x)), \\
    %    \item \textbf{Natural language description}:
    %   \text{There is a dog which is seen by John.}
    % \end{itemize}
% \end{enumerate}

\subsection{Different Tasks Performance}
Furthermore, we conducted an in-depth analysis of the specific performance of various SR across different tasks, as summarized in the Table \ref{tab:dif_task_per}. To explore the relationship between task types and the effectiveness of SR, we categorized the 10 tasks into three groups: (1) tasks with overall negative impact, (2) tasks with partial effectiveness (effectiveness ratio below 50\%), and (3) tasks with predominant effectiveness (effectiveness ratio above 50\%). We will analyze them one by one based on the characteristics of the task.

First, let's go with the tasks with Overall Negative Impact (including Logic, AGNEWS, and CoNLL2003):
\begin{itemize}
  \item Logical Fallacy Detection. This task primarily relies on analyzing argument structures and intuitively understanding logical relationships, rather than solely depending on syntactic or semantic information. Although AMR, FOL, and PST can provide structural, logical, and semantic information of sentences, they cannot directly reveal the logical validity of arguments or the interrelations between different propositions.
  \item News Classification. Classification in this task is primarily based on the topic and context of the content. While syntactic and semantic information aids in understanding sentence structure, the classification usually hinges on the extraction of key information and the rapid identification of themes, rather than complex linguistic analysis. Effective classification often requires the integration of background knowledge and domain-specific features, which go beyond the scope of syntactic and semantic representations.
  \item Named Entity Recognition (NER). NER necessitates the precise identification of specific entities within the text. Although PST can provide structural information about words, entity recognition typically depends on context and specific naming patterns, which may not be adequately captured by syntactic information alone. Similarly, adding semantic and logical information does not significantly improve performance in this context.
\end{itemize}

Next is the Partial Effectiveness(including PAWS, Pubmed45, WiC, and WMT16):
\begin{itemize}
  \item PAWS. The combination of AMR and FOL resulted in a significant performance improvement of 9.24\%, while combinations involving PST exhibited a noticeable decline. In paraphrase detection, the model needs to discern semantic similarities between sentences. The semantic and logical information provided by AMR and FOL helps capture the core meaning of sentences, thereby enhancing the model’s understanding. However, when sentences have similar syntactic structures but subtle semantic differences, the model may incorrectly identify them as equivalent due to PST similarities, leading to performance degradation.
  \item Pubmed45. This task primarily involves event extraction, which relies on understanding the semantic relationships and contextual information within biomedical texts. Successful event extraction requires a deep understanding of text semantics and accurate identification of event components. The introduction of logical information might distract the model from focusing on specific event features and context, thereby disrupting the extraction process and explaining why FOL underperformed in this task.
  \item WiC. In this task, the model's decision-making hinges on the precise understanding and disambiguation of words within context. The model must determine the different meanings of a word based on varying contexts, making a deep comprehension of semantics essential. Therefore, the addition of extra semantic information (AMR) significantly improved the overall performance.
  \item WMT16. Translation tasks require the model to convert source language texts into target languages while maintaining the original meaning and tone. The model must handle syntactic and semantic information in the source language, as well as address structural differences, grammatical rules, and logical information between languages to ensure accurate and natural translation. Although additional prompts can aid semantic understanding, the model predominantly relies on its internal translation rules and language capabilities in this task, making the marginal effect of extra information relatively minor.
\end{itemize}

Last is the Predominant Effectiveness (including SNLI, SST-2, and SPIDER):
\begin{itemize}
  \item SNLI. In this task, the model must assess entailment relationships between sentence pairs (i.e., whether one sentence can be inferred from another). The structured information provided by AMR, PST, and FOL helps the model better understand the logical and semantic relationships between sentences, particularly when dealing with complex sentence structures. This information clarifies the subject, predicate, and object within sentences and their interrelations, thereby enhancing the model’s ability to judge entailment relationships.
  \item Sentiment Analysis. This task requires the model to determine the emotional orientation of the text. While the model's performance was suboptimal with original structured information, using NLD provided clearer guidance in terms of semantics, logic, and syntax, enabling the model to better comprehend the sentiment expressed in the text, which led to substantial performance improvement.
  \item SPIDER. This task involves converting natural language queries into SQL statements, a more complex task than sentiment analysis. When faced with diverse queries and complex database structures, the model is more likely to encounter comprehension difficulties. In such cases, structured information provides the model with a clear context and logical relationships concerning the queries, facilitating the identification of key components and the target database tables. This transformation significantly improves the accuracy of SQL generation, particularly for complex queries, resulting in notable performance gains.
\end{itemize}

% \begin{figure}[h!]
% \centering
% % \vspace{-0.9cm}
% \includegraphics[width=0.8\linewidth]{picture/图片4.png}
% % \vspace{-0.5cm}
% \caption{
% % \KY{I still find the teaser not easy to understand. WHat is your message? Can you write them down so to see your point?
% % Also, current introduction has no relation with the introduction. I think it is not okay.}
% }
% \label{fig:图片4}
% % \vspace{-0.3cm}
% \end{figure}

\setlength{\tabcolsep}{4.5pt}
\renewcommand{\arraystretch}{1.2}
\begin{table*}[]
\centering
\vspace{-0.1in}
\caption{Differ Task Performance.}
\label{tab:dif_task_per}
\vspace{0.05in}
% \small
\tiny
\begin{tabular}{cccc |
>{\columncolor[HTML]{FFFFFF}}c 
>{\columncolor[HTML]{FFFFFF}}c 
>{\columncolor[HTML]{FFFFFF}}c 
>{\columncolor[HTML]{FFFFFF}}c 
>{\columncolor[HTML]{FFFFFF}}c 
>{\columncolor[HTML]{FFFFFF}}c 
>{\columncolor[HTML]{FFFFFF}}c 
>{\columncolor[HTML]{FFFFFF}}c 
>{\columncolor[HTML]{FFFFFF}}c 
>{\columncolor[HTML]{FFFFFF}}c }
\toprule
\multicolumn{1}{l}{\textbf{AMR}} & \multicolumn{1}{l}{\textbf{PST}} & \multicolumn{1}{l}{\textbf{FOL}} & \multicolumn{1}{l|}{\textbf{NLD}} & \textbf{Logic}                                    & \textbf{AGNEWS}                                  & \textbf{CoNLL}                                & \textbf{PAWS}                                     & \textbf{Pubmed45}                                 & \textbf{WiC}                                      & \textbf{WMT16}                                   & \textbf{SNLI}                                    & \textbf{SST-2}                                   & \textbf{SPIDER}                                  \\
\midrule
\checkmark                       &                         &                         &                         & {\color[HTML]{F54A45} -6.04\%}                    & {\color[HTML]{F54A45} -4.92\%}                   & {\color[HTML]{F54A45} -6.64\%}                    & {\color[HTML]{F54A45} -2.92\%}                    & {\color[HTML]{F54A45} -1.69\%}                    & {\color[HTML]{F54A45} -1.89\%}                    & {\color[HTML]{F54A45} -3.08\%}                   & {\color[HTML]{F54A45} -2.46\%}                   & {\color[HTML]{F54A45} -5.59\%}                   & {\color[HTML]{F54A45} -6.04\%}                   \\
                        & \checkmark                       &                         &                         & {\color[HTML]{F54A45} -7.95\%}                    & {\color[HTML]{F54A45} \textit{\textbf{-8.73\%}}} & {\color[HTML]{F54A45} -4.77\%}                    & {\color[HTML]{F54A45} -7.64\%}                    & {\color[HTML]{F54A45} -4.12\%}                    & {\color[HTML]{F54A45} -6.88\%}                    & {\color[HTML]{F54A45} -2.06\%}                   & {\color[HTML]{F54A45} \textit{\textbf{-5.97\%}}} & {\color[HTML]{F54A45} -2.03\%}                   & {\color[HTML]{34C724} 0.58\%}                    \\
                        &                         & \checkmark                       &                         & {\color[HTML]{F54A45} -2.78\%}                    & {\color[HTML]{F54A45} -2.90\%}                   & {\color[HTML]{F54A45} -4.16\%}                    & {\color[HTML]{34C724} 0.48\%}                     & {\color[HTML]{F54A45} \textit{\textbf{-11.42\%}}} & {\color[HTML]{F54A45} \textit{\textbf{-16.58\%}}} & {\color[HTML]{F54A45} -2.50\%}                   & {\color[HTML]{F54A45} -3.72\%}                   & {\color[HTML]{34C724} 0.26\%}                    & {\color[HTML]{F54A45} -1.12\%}                   \\
\checkmark                       & \checkmark                       &                         &                         & {\color[HTML]{F54A45} -12.65\%}                   & {\color[HTML]{F54A45} -5.42\%}                   & {\color[HTML]{F54A45} -8.42\%}                    & {\color[HTML]{F54A45} \textit{\textbf{-11.66\%}}} & {\color[HTML]{34C724} 1.11\%}                     & {\color[HTML]{F54A45} -6.99\%}                    & {\color[HTML]{F54A45} -1.85\%}                   & {\color[HTML]{F54A45} -5.13\%}                   & {\color[HTML]{F54A45} -6.62\%}                   & {\color[HTML]{F54A45} -3.66\%}                   \\
\checkmark                       &                         & \checkmark                       &                         & {\color[HTML]{F54A45} -8.53\%}                    & {\color[HTML]{F54A45} -5.41\%}                   & {\color[HTML]{F54A45} -8.60\%}                    & {\color[HTML]{34C724} 2.57\%}                     & {\color[HTML]{F54A45} -4.71\%}                    & {\color[HTML]{F54A45} -9.46\%}                    & {\color[HTML]{F54A45} \textit{\textbf{-3.73\%}}} & {\color[HTML]{F54A45} -0.94\%}                   & {\color[HTML]{F54A45} -6.33\%}                   & {\color[HTML]{F54A45} \textit{\textbf{-6.52\%}}} \\
                        & \checkmark                       & \checkmark                       &                         & {\color[HTML]{F54A45} -7.80\%}                    & {\color[HTML]{F54A45} -5.98\%}                   & {\color[HTML]{F54A45} -8.30\%}                    & {\color[HTML]{F54A45} -5.46\%}                    & {\color[HTML]{F54A45} -0.58\%}                    & {\color[HTML]{F54A45} -15.10\%}                   & {\color[HTML]{F54A45} -1.28\%}                   & {\color[HTML]{34C724} 0.26\%}                    & {\color[HTML]{F54A45} \textit{\textbf{-8.64\%}}} & {\color[HTML]{F54A45} -4.26\%}                   \\
\checkmark                       & \checkmark                       & \checkmark                       &                         & {\color[HTML]{F54A45} \textit{\textbf{-13.44\%}}} & {\color[HTML]{F54A45} -3.52\%}                   & {\color[HTML]{F54A45} \textit{\textbf{-11.75\%}}} & {\color[HTML]{F54A45} -4.84\%}                    & {\color[HTML]{F54A45} -7.26\%}                    & {\color[HTML]{F54A45} -9.04\%}                    & {\color[HTML]{F54A45} -3.09\%}                   & {\color[HTML]{34C724} 0.22\%}                    & {\color[HTML]{F54A45} -5.36\%}                   & {\color[HTML]{F54A45} -5.49\%}                   \\
\checkmark                       &                         &                         & \checkmark                       & {\color[HTML]{F54A45} -4.06\%}                    & {\color[HTML]{F54A45} -1.18\%}                   & {\color[HTML]{F54A45} -4.38\%}                    & {\color[HTML]{34C724} 0.71\%}                     & {\color[HTML]{F54A45} -0.65\%}                    & {\color[HTML]{34C724} \textit{\textbf{4.46\%}}}   & {\color[HTML]{F54A45} -3.26\%}                   & {\color[HTML]{34C724} 4.75\%}                    & {\color[HTML]{34C724} 0.84\%}                    & {\color[HTML]{34C724} \textit{\textbf{6.51\%}}}  \\
                        & \checkmark                       &                         & \checkmark                       & {\color[HTML]{F54A45} -5.61\%}                    & {\color[HTML]{F54A45} -3.91\%}                   & {\color[HTML]{F54A45} -6.14\%}                    & {\color[HTML]{F54A45} -11.27\%}                   & {\color[HTML]{F54A45} -0.65\%}                    & {\color[HTML]{F54A45} -3.30\%}                    & {\color[HTML]{34C724} 2.53\%}                    & {\color[HTML]{34C724} 6.87\%}                    & {\color[HTML]{34C724} 0.95\%}                    & {\color[HTML]{34C724} 4.67\%}                    \\
                        &                         & \checkmark                       & \checkmark                       & {\color[HTML]{F54A45} -2.52\%}                    & {\color[HTML]{F54A45} -1.94\%}                   & {\color[HTML]{F54A45} -3.11\%}                    & {\color[HTML]{34C724} 5.86\%}                     & {\color[HTML]{F54A45} -10.33\%}                   & {\color[HTML]{34C724} 4.26\%}                     & {\color[HTML]{34C724} 1.66\%}                    & {\color[HTML]{34C724} 3.95\%}                    & {\color[HTML]{34C724} 1.52\%}                    & {\color[HTML]{34C724} 3.80\%}                    \\
\checkmark                       & \checkmark                       &                         & \checkmark                       & {\color[HTML]{F54A45} -5.61\%}                    & {\color[HTML]{F54A45} -3.76\%}                   & {\color[HTML]{F54A45} -1.72\%}                    & {\color[HTML]{F54A45} -11.11\%}                   & {\color[HTML]{34C724} \textit{\textbf{3.47\%}}}   & {\color[HTML]{F54A45} -3.61\%}                    & {\color[HTML]{F54A45} -2.28\%}                   & {\color[HTML]{34C724} \textit{\textbf{8.89\%}}}  & {\color[HTML]{34C724} 1.64\%}                    & {\color[HTML]{34C724} 5.32\%}                    \\
\checkmark                       &                         & \checkmark                       & \checkmark                       & {\color[HTML]{F54A45} -4.94\%}                    & {\color[HTML]{F54A45} -4.15\%}                   & {\color[HTML]{F54A45} -4.10\%}                    & {\color[HTML]{34C724} \textit{\textbf{9.24\%}}}   & {\color[HTML]{34C724} 2.61\%}                     & {\color[HTML]{F54A45} -3.54\%}                    & {\color[HTML]{F54A45} -1.22\%}                   & {\color[HTML]{34C724} 8.40\%}                    & {\color[HTML]{34C724} 2.79\%}                    & {\color[HTML]{34C724} 4.88\%}                    \\
                        & \checkmark                       & \checkmark                       & \checkmark                       & {\color[HTML]{F54A45} -5.59\%}                    & {\color[HTML]{F54A45} -4.25\%}                   & {\color[HTML]{F54A45} -2.66\%}                    & {\color[HTML]{F54A45} -6.77\%}                    & {\color[HTML]{34C724} 0.35\%}                     & {\color[HTML]{F54A45} -6.88\%}                    & {\color[HTML]{34C724} 1.34\%}                    & {\color[HTML]{34C724} 3.74\%}                    & {\color[HTML]{34C724} \textit{\textbf{3.85\%}}}  & {\color[HTML]{34C724} 5.01\%}                    \\
\checkmark                       & \checkmark                       & \checkmark                       & \checkmark                       & {\color[HTML]{F54A45} -9.17\%}                    & {\color[HTML]{F54A45} -4.28\%}                   & {\color[HTML]{F54A45} -3.77\%}                    & {\color[HTML]{F54A45} -1.99\%}                    & {\color[HTML]{34C724} 2.81\%}                     & {\color[HTML]{F54A45} -2.51\%}                    & {\color[HTML]{34C724} \textit{\textbf{2.71\%}}}  & {\color[HTML]{34C724} 4.50\%}                    & {\color[HTML]{34C724} 1.74\%}                    & {\color[HTML]{34C724} 4.28\%}                   \\
\bottomrule
\end{tabular}
\end{table*}

\subsection{LAUD}
\begin{figure*}[h!]
\centering
\vspace{-0.1in}
\includegraphics[width=\linewidth]{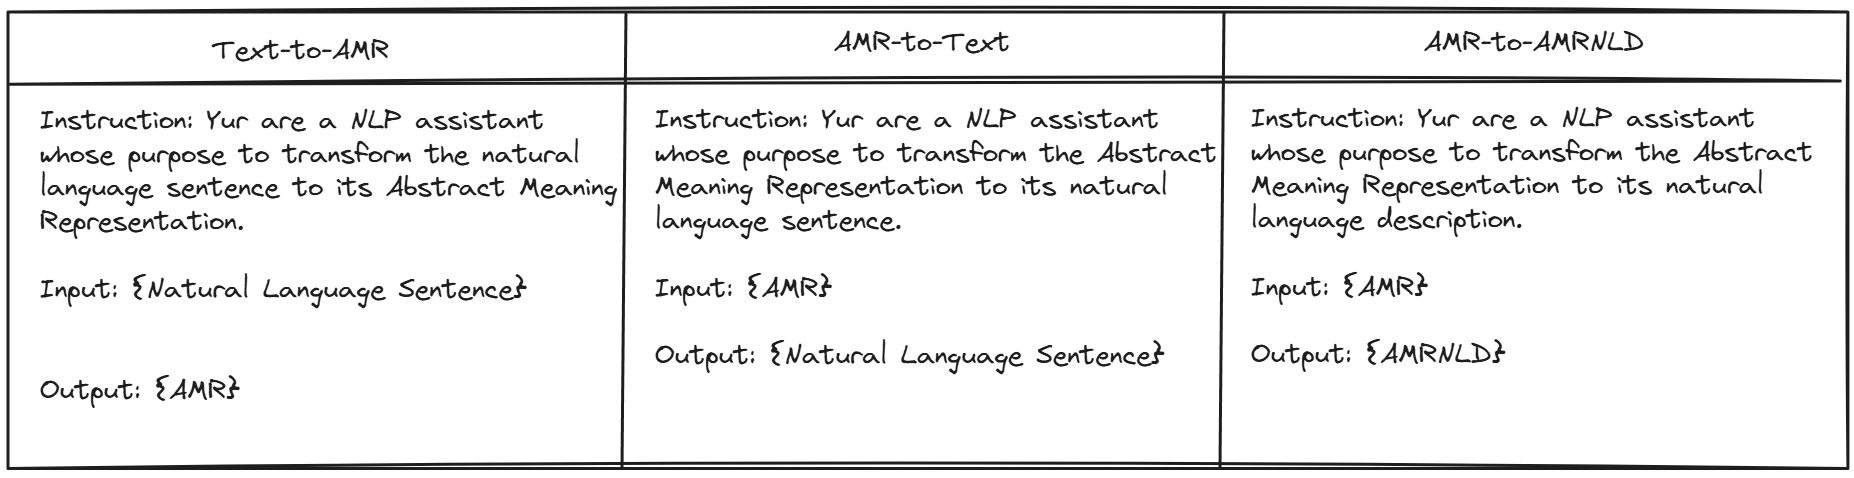}
% \vspace{-0.2in}
\caption{Trainig Set Example.}
\label{fig:traing_set_example}
\vspace{-0.1in}
\end{figure*}

Subsequently, we aimed to enhance the overall understanding of AMR data by the LLM to examine whether improved comprehension of this structured representation could boost reasoning capabilities without task-specific Fine-Tuning. To this end, we designed two training datasets. The first dataset comprises two tasks: AMR-to-Text and Text-to-AMR, each containing 50,000 samples. The second dataset builds upon the first by adding the AMR-to-AMRNLD task, with each task also containing 50,000 samples. Specific examples of these tasks are illustrated in the Figure \ref{fig:traing_set_example}.
The Table\ref{tab:differ_nlp_laud} presents the model's performance across five NLP tasks. It can be observed that, compared to the AMRCOT and BASE strategies, which directly query the LLM, the use of AMR generally had a significantly negative impact on performance across. This discrepancy with the earlier experimental results made us to conduct further investigations during the pretraining stage.


\setlength{\tabcolsep}{5pt}
\renewcommand{\arraystretch}{1.2}
\begin{table*}[]
\centering
\vspace{-0.1in}
\caption{Differ NLP LAUD.}
\label{tab:differ_nlp_laud}
\vspace{0.05in}
\small
\begin{tabular}{l|c|ccccc}
\toprule
\textbf{model}                    & \textbf{prompt\_strategy} & \textbf{PAWS}                   & \textbf{Logic}                  & \textbf{Pubmed45}               & \textbf{SPIDER}                 & \textbf{WMT16}                  \\
\midrule
                                  & base                      & 0.516                           & 0.195                           & 0.383                           & 0.278                           & 0.132                           \\
                                  & AMRCOT                    & 0.366                           & 0.161                           & 0.341                           & 0.246                           & 0.125                           \\
\multirow{-3}{*}{base}            & ${\Delta}_{AMRCOT}$                   & {\color[HTML]{FF0000} -29.00\%} & {\color[HTML]{FF0000} -17.41\%} & {\color[HTML]{FF0000} \textbf{-11.12}\%} & {\color[HTML]{FF0000} \textbf{-11.51}\%} & {\color[HTML]{FF0000} \textbf{-4.98}\%}  \\
\hline
                                  & base                      & 0.532                           & 0.213                           & 0.396                           & 0.298                           & 0.107                           \\
                                  & AMRCOT                    & 0.408                           & 0.184                           & 0.216                           & 0.172                           & 0.046                           \\
\multirow{-3}{*}{a2t \& t2a}        & ${\Delta}_{AMRCOT}$                   & {\color[HTML]{FF0000} -23.31\%} & {\color[HTML]{FF0000} -13.62\%} & {\color[HTML]{FF0000} -45.45\%} & {\color[HTML]{FF0000} -42.28\%} & {\color[HTML]{FF0000} -57.01\%} \\
\hline
                                  & base                      & 0.591                           & 0.151                           & 0.393                           & 0.276                           & 0.103                           \\
                                  & AMRCOT                    & 0.519                           & 0.165                           & 0.146                           & 0.242                           & 0.045                           \\
\multirow{-3}{*}{a2t \& t2a \& a2nld} & ${\Delta}_{AMRCOT}$                   & {\color[HTML]{FF0000} \textbf{-12.16}\%} & {\color[HTML]{00B050} \textbf{8.89}\%}   & {\color[HTML]{FF0000} -62.83\%} & {\color[HTML]{FF0000} -12.32\%} & {\color[HTML]{FF0000} -56.13\%} \\
\bottomrule
\end{tabular}
\end{table*}


\subsection{Full Result}
We initially focused our investigation on the performance of the relatively weaker model, GPT-3.5-turbo. Figure \ref{fig:gpt_35_color_map} illustrates the comparative results of incorporating various SR and their corresponding Natural Language Descriptions (SRNLD). Each cell in the figure represents the performance improvement ($\Delta I$) associated with a specific prompt. The intensity of the purple color indicates the extent of performance enhancement, with darker shades signifying greater improvements. Conversely, darker shades of blue indicate a more significant decline in performance. The results reveal that the use of SRNLD leads to a considerably higher proportion of purple cells compared to the use of original SR, which aligns with our prior observations and hypotheses. Specifically, for less capable LLMs like GPT-3.5-turbo, there is a noticeable challenge in comprehending and leveraging complex and abstract structured representations. However, when these representations are transformed into natural language forms that are more familiar to LLMs, the models are better equipped to utilize this information, resulting in superior performance across most downstream tasks compared to using the original text alone.

\begin{figure*}
\centering
\vspace{0in}
\includegraphics[width=\linewidth]{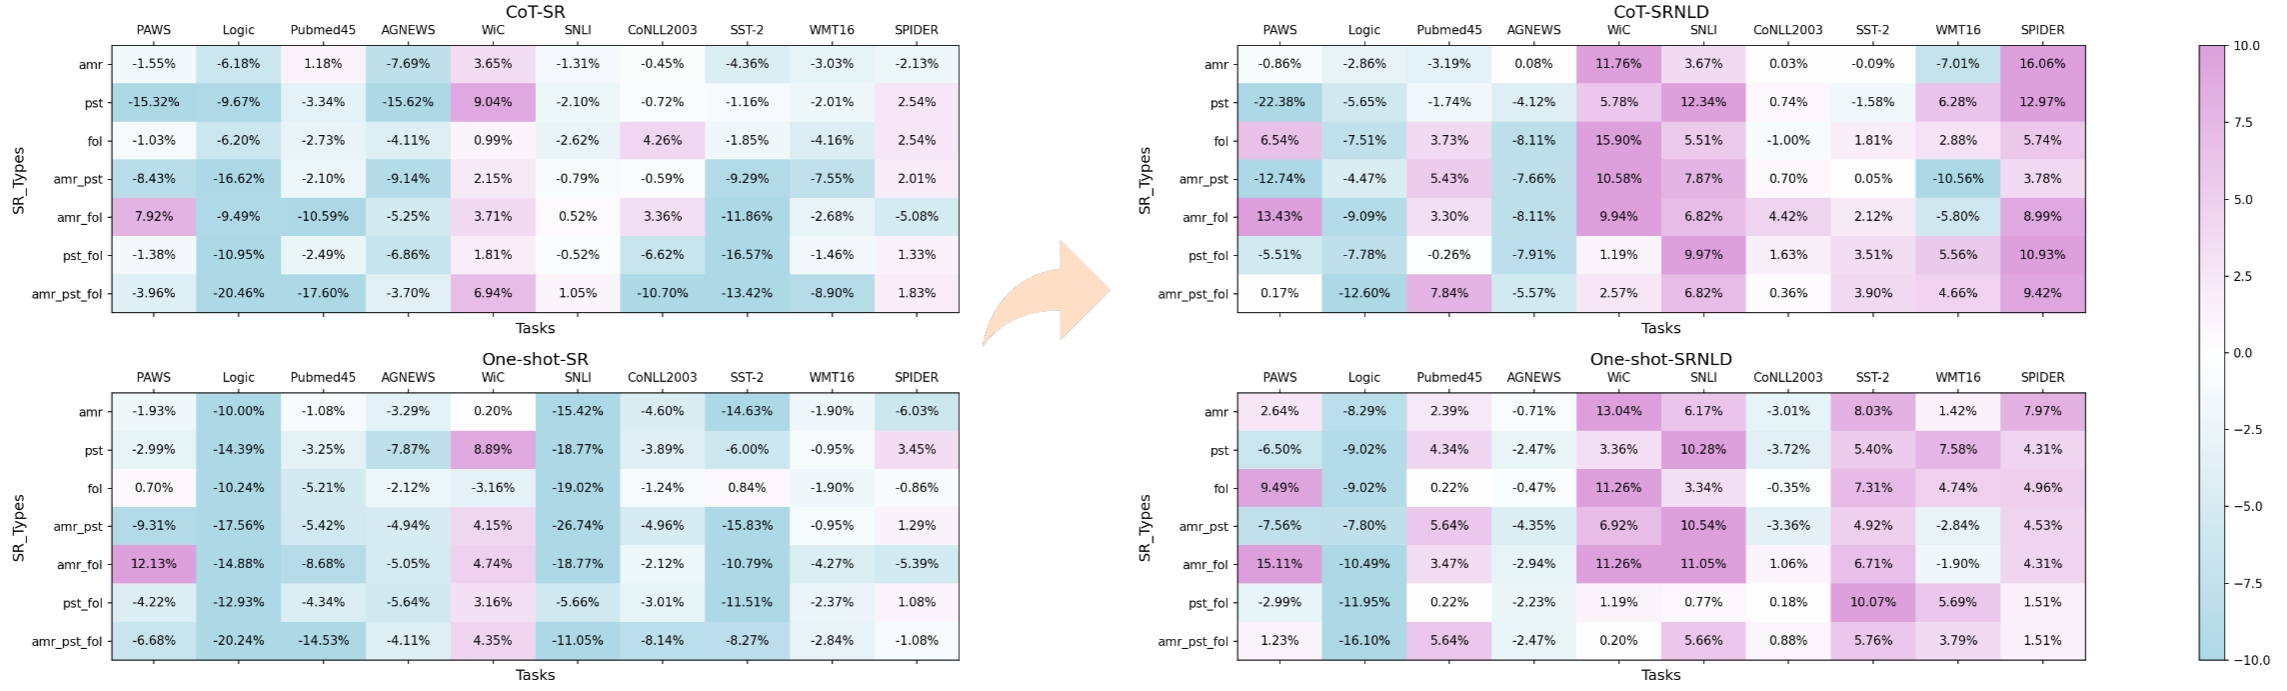}
% \vspace{-0.2in}
\caption{GPT-3.5-turbo Performance}
\label{fig:gpt_35_color_map}
\vspace{-0.1in}
\end{figure*}


Next, we conducted an in-depth analysis of the performance of different SR, with the average performance improvement across all tasks summarized in the Table \ref{tab:dif_sr_per}. The results indicate that the use of individual SRs such as AMR, PST, and FOL did not lead to significant performance enhancements, which is consistent with the findings of \cite{jin2024analyzing}. Moreover, when multiple SRs were introduced simultaneously, their combined complexity posed additional challenges for the LLMs, further dispersing the model’s attention and resulting in poorer performance compared to using a single SR. In contrast, when relatively weaker LLMs were provided with more comprehensible semantic features (AMR) and logical features (FOL), their average performance improved. The integration of these two types of features complemented each other, leading to better overall results. However, the contribution of syntactic features (PST) was relatively less effective and, in some cases, even negated the positive effects of semantic and logical features.



\setlength{\tabcolsep}{12.0pt}
\renewcommand{\arraystretch}{1.2}
\begin{table*}[]
\centering
\vspace{-0.05in}
\caption{Differ SR Performance.}
\label{tab:dif_sr_per}
\vspace{0.05in}
\small
\begin{tabular}{ccc|cc|cc}
\toprule
\multicolumn{1}{c}{}                               & \multicolumn{1}{c}{}                               & \multicolumn{1}{c}{}                               & \multicolumn{2}{|c|}{\textbf{4o-mini}}                                                                & \multicolumn{2}{c}{\textbf{3.5 turbo}}                                                             \\
% \cline{4-7}
\multicolumn{1}{c}{\multirow{-2}{*}{\textbf{AMR}}} & \multicolumn{1}{c}{\multirow{-2}{*}{\textbf{PST}}} & \multicolumn{1}{c|}{\multirow{-2}{*}{\textbf{FOL}}} & $\overline{{\Delta}_{SR}}$                                     & $\overline{{\Delta}_{SRNLD}}$                                  & $\overline{{\Delta}_{SR}}$                                     & $\overline{{\Delta}_{SRNLD}}$                                 \\
\midrule
\checkmark                                                  &                                                    &                                                    & {\color[HTML]{F54A45} \textit{\textbf{-4.23\%}}}                   & {\color[HTML]{F54A45} -1.62\%}                   & {\color[HTML]{F54A45} -4.03\%}                   & {\color[HTML]{34C724} 2.37\%}                   \\
                                                   & \checkmark                                                  &                                                    & {\color[HTML]{F54A45} -5.71\%}                   & {\color[HTML]{F54A45} -3.98\%}                   & {\color[HTML]{F54A45} -4.21\%}                   & {\color[HTML]{34C724} 0.82\%}                   \\
                                                   &                                                    & \checkmark                                                  & {\color[HTML]{F54A45} -6.03\%}                   & {\color[HTML]{F54A45} -2.22\%}                   & {\color[HTML]{F54A45} \textit{\textbf{-2.86\%}}}                   & {\color[HTML]{34C724} 2.85\%}                   \\
\checkmark                                                  & \checkmark                                                  &                                                    & {\color[HTML]{F54A45} -5.73\%}                   & {\color[HTML]{F54A45} -1.74\%}                   & {\color[HTML]{F54A45} -6.53\%}                   & {\color[HTML]{F54A45} -0.02\%}                  \\
\checkmark                                                  &                                                    & \checkmark                                                  & {\color[HTML]{F54A45} -6.21\%}                   & {\color[HTML]{F54A45} \textit{\textbf{-1.19\%}}}                   & {\color[HTML]{F54A45} -4.13\%} & {\color[HTML]{34C724} \textit{\textbf{3.19\%}}} \\
                                                   & \checkmark                                                  & \checkmark                                                  & {\color[HTML]{F54A45} -6.97\%} & {\color[HTML]{F54A45} -3.07\%}                   & {\color[HTML]{F54A45} -4.46\%}                   & {\color[HTML]{34C724} 0.69\%}                   \\
\checkmark                                                  & \checkmark                                                  & \checkmark                                                  & {\color[HTML]{F54A45} -5.64\%}                   & {\color[HTML]{F54A45} -2.32\%} & {\color[HTML]{F54A45} -7.08\%}                   & {\color[HTML]{34C724} 1.19\%}       \\
\bottomrule
\end{tabular}
\end{table*}


\paragraph{Conclusion}
\begin{itemize}
  \item The utilization of SRNLD has demonstrated the potential to improve the performance of less capable models. 
Overall, SRNLD outperforms original SR, as the transformed natural language descriptions are more comprehensible and usable for the models compared to the original structured forms.
  \item The combination of semantic and logical features is particularly effective: the integration of AMR and FOL contributes to performance improvements. However, the inclusion of syntactic features, such as PST, may counteract these benefits.
  \item SR (e.g., AMR and FOL) significantly enhance model performance in tasks involving logical reasoning, complex semantic understanding, and structured tasks such as SQL generation. Conversely, in tasks that heavily depend on contextual understanding or key information extraction, such as news classification and named entity recognition, the additional information provided by SR can become redundant and may disrupt the model's judgment, ultimately leading to performance degradation.
\end{itemize}



\setlength{\tabcolsep}{4.5pt}
\renewcommand{\arraystretch}{1.2}
\begin{table}[h!]
\centering
\vspace{-0.1in}
\caption{Tasks and datasets used}
\label{tab:dataset_of_prompt}
\vspace{-0.1in}
\small
\resizebox{0.5\textwidth}{!}
{ 
\begin{tabular}{lcc}
\toprule
\textbf{Dataset} & \textbf{Task} & \textbf{Test Size} \\
\midrule
PAWS      & Paraphrase Detection          & 8000  \\
SNLI      & Recognizing Textual Entailment & 10000 \\
WMT16     & Translation                   & 5999  \\
CoNLL2003 & Named Entity Recognition       & 3453  \\
Logic     & Logical Fallacy Detection     & 2449  \\
SST-2     & Sentiment Analysis            & 872   \\
Pubmed45  & Event Extraction              & 5000  \\
WiC       & Lexical Disambiguation        & 1438  \\
SPIDER    & Text2SQL Code Generation      & 8034  \\
AGNEWS    & Text Classification           & 7600  \\
\bottomrule
\end{tabular}
} 
\vspace{-0.1in}
\end{table}



To further investigate this, I selected five tasks for additional experiments, adjusting the ratio of text to structured representations in the Gen-SR dataset to identify the optimal balance. The experimental results are shown in the Figure~\ref{fig:dif_weight}. As can be observed, the fluctuations in performance with different ratios are relatively small. For both AMR and PST, a 50-50 ratio between text and structured representations appears to be the most effective. However, for FOL, a 30-70 ratio (favoring structured representations) yields better results. This is a preliminary exploration, and I believe it represents a promising direction for further research.

\begin{figure}[h!]
\centering
\vspace{-0.1in}
\includegraphics[width=\linewidth]{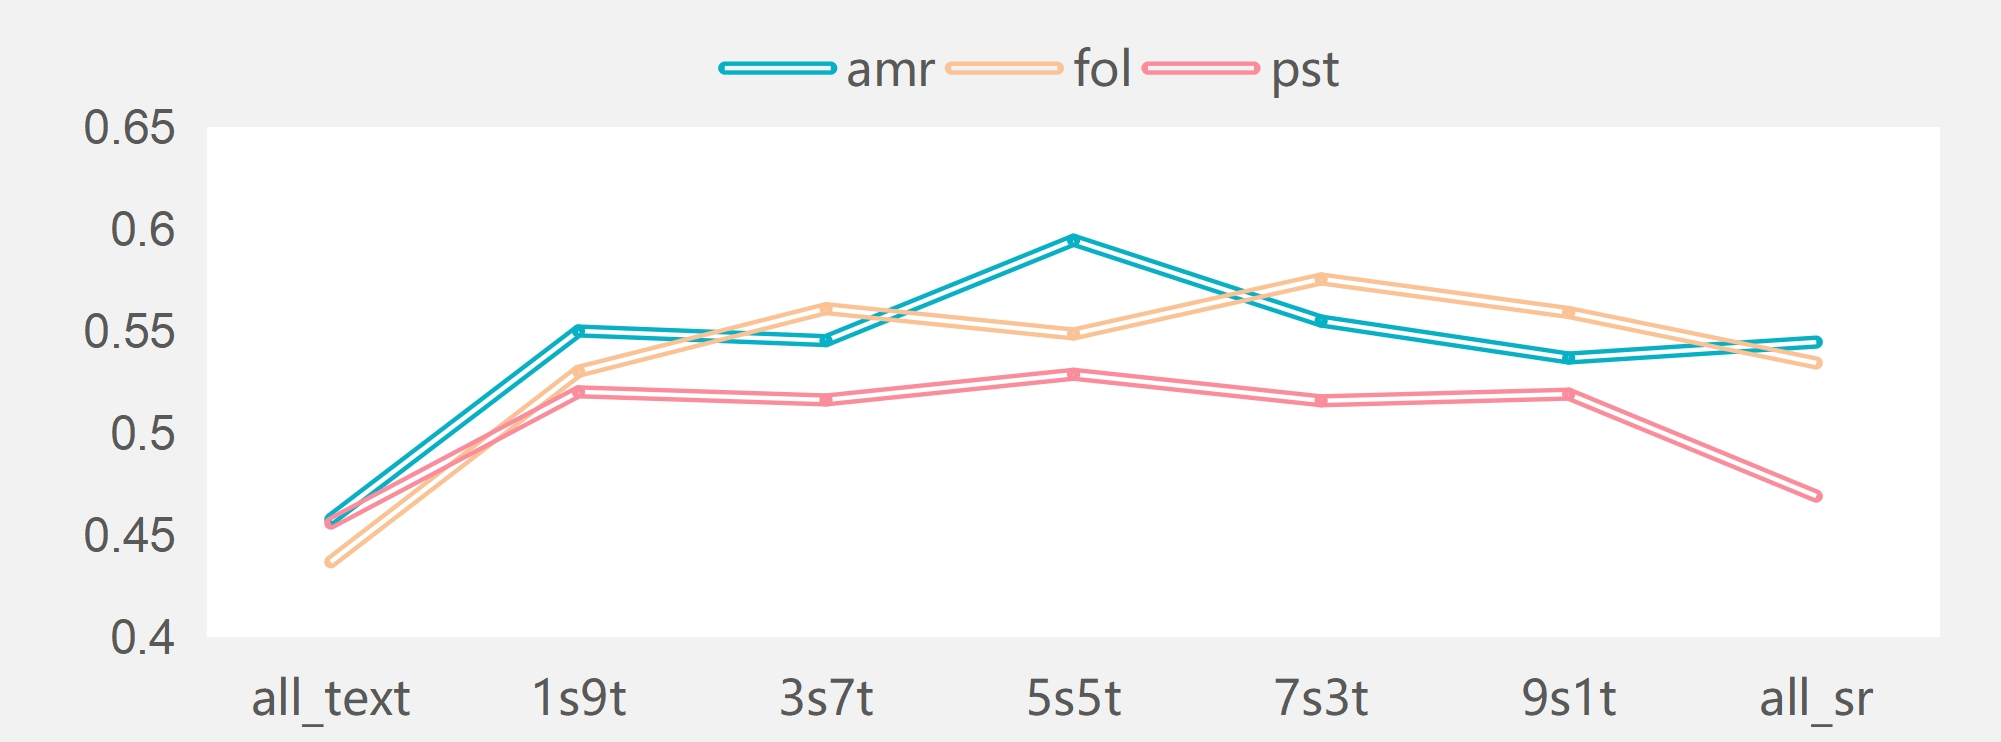}
% \vspace{-0.2in}
\caption{Differ Weight.}
\label{fig:dif_weight}
\vspace{-0.1in}
\end{figure}
